# Supplementary material for: High Performance Data Persistence in Non-Volatile Memory for Resilient High Performance Computing
Source: arXiv:1705.00264 source file (2017-05-02)
Supplement: Supplementary file 1 [file artifacts-appendix-sc17.pdf]

# A. Artifact Description: High Performance Data Persistence in Non-Volatile Memory for Resilient High Performance Computing

## A.1 Abstract

In our SC'17 submission, we investigate whether non-volatile memory (NVM) based checkpoint can be performed frequently to improve HPC system resilience and reduce re-computation cost. We further introduce a technique, named *in-place versioning*, to avoid data copying inherent in checkpoint to improve performance. We also optimize cache flushing performance to enable data consistence between NVM and caches.

In this appendix, we describe some details for how to perform cache flushing, how we emulate NVM, how the benchmarks used in the paper are transformed to implement the in-place versioning, and where we insert a few APIs in benchmarks to trigger asynchronous and proactive cache flushing.

## A.2 Description

### A.2.1 Check-list (artifact meta information)

- **Algorithm:** The paper describes in details the in-place versioning that leverages application inherent write operations to create data copy and maintain persistence with consistence in NVM. The paper also describes an asynchronous and proactive cache flushing algorithm.
- **Program:** A runtime library that enables asynchronous and proactive cache flushing, a kernel module that allows applications to indirectly use the privileged cache flushing instruction, and an LLVM-based code transformation tool.
- **Compilation:** GCC4.4.7, LLVM3.4, GNU Make, OpenMPI1.10 and GCC4.6 (for Dragonegg).
- **Transformations:** in-place versioning
- **Binary:** -
- **Data set:** Public available benchmarks: NPB3.3.1, Nek5000
- **Run-time environment:** Linux system. To load our kernel module, the privileged accesses to the system is required.
- **Hardware:** Any x86 processors that support CLFLUSH, WBINVD and SSE2 instructions. Standalone or Multi-machines.
- **Run-time state:** The system is idle and only running our tests.
- **Output:** Execution result correctness and performance reported by the benchmarks.
- **Experiment workflow:** See below.
- **Experiment customization:** Increase problem size of eddy for Nek5000. See below
- **Publicly available?:** Some code are available, but not all.

### A.2.2 How software can be obtained

`https://gitlab.com/sc17hpc/HPDP_NVM`

includes some of our code.

**Table 1.** Hardware configurations

| Hardware | **LBNL Edison** | **Local clusters** |
|---|---|---|
| Nodes | 4 | 4 |
| Dram | DDR3 64GB | DDR4 32GB |
| CPU | Intel(R) Ivy bridge | Intel(R) Xeon(R) CPU E5-2630 v3 @ 2.40GHz |
| Cache: L1-L2-L3 | 32K-256K-30M | 32K-256K-20M |
| Privilege access | NO | YES |

### A.2.3 Hardware dependencies

Any x86 multicore CPU that supports CLFLUSH,WBINVD and SSE2 instructions. Standalone or Multi-machine

### A.2.4 Software dependencies

- **LLVM-based dynamic instruction trace generation tool (LLVM-Tracer):** https://github.com/ysshao/LLVM-Tracer
- **Quartz:** DRAM based performance emulator for NVM. Quartz is deployed on a local cluster to emulate a heterogeneous NVM/DRAM system with NVM configured with 1/8 DRAM bandwidth and DRAM configured with 256MB capacity to enable a practical emulation of NVM. We need to use the bandwidth model when using Quartz. To configure the bandwidth parameter in Quartz, one must set concrete memory latency or bandwidth numbers in *nvmemul.ini* file. The follow is the configuration we use to emulate 1/8 DRAM bandwidth:
  - bandwidth:
    {
    enable = false; //use the bandwidth model
    model = "/tmp/bandwidth_model";
    read = 2000;
    write = 2000;
    };

To emulate a heterogeneous NVM/DRAM system, one must have a machine with at least two NUMA nodes. One NUMA node is used as regular DRAM, and the other NUMA node is controlled by the Quartz emulator to change memory bandwidth.

### A.2.5 Datasets

- **NPB3.3.1:** Public available at https://www.nas.nasa.gov/assets/npb/NPB3.3.1.tar.gz. Class C and D are used.
  Edit NPB3.3.1-MPI/config/make.def to change compiler, linkage flag setting.
- **Nek5000:**Public available at https://github.com/Nek5000/Nek5000.
  Add Nek5000/bin to environemnt variables $PATH
- **NekExample_Eddy:**Public available at https://github.com/Nek5000/NekExamples/tree/master/eddy.

## A.3 Installation

- Install Quartz:Please follow their official instructions. sudo permission is required. (https://github.com/HewlettPackard/quartz).
- Install our WBINVD kernel module.

```
cd wbinvd && make all && sudo insmod wbinvd.ko
```

```
1   asm volatile ("CPUID\n\t" "RDTSC\n\t"
2       "mov %%edx, %0\n\t"
3       "mov %%eax, %1\n\t":
4       "=r" (cycles_high), "=r" (cycles_low)::
5       "%rax", "%rbx", "%rcx", "%rdx");
6   //Instructions to be measured.
7   flush(addr);
8   asm volatile("RDTSCP\n\t"
9       "mov %%edx, %0\n\t"
10      "mov %%eax, %1\n\t"
11      "CPUID\n\t": "=r" (cycles_high1),
12      "=r" (cycles_low1)::
13      "%rax", "%rbx", "%rcx", "%rdx");
14  start = ( ((uint64_t)cycles_high << 32) |
    cycles_low );
15  end = ( ((uint64_t)cycles_high1 << 32) |
    cycles_low1 );
16  printf("%"PRIu64" clock cycles\n\n", (end-
    start));
17
```

**Figure 1.** Accurately measure clflush performance.

A file named *wbinvd* will be create in /proc/. Whenever *wbinvd* is opened, the privilege instruction *wbinvd*() will be executed to trigger system wide cache flushing.

- Install the perf utility: We use perf to collect system wide cache misses for performance evaluation. Use the following to install it on an Ubuntu system.

```
apt-get install linux-tools-common \
linux-tools-generic linux-tools-`uname -r`
```

### A.4 Evaluation and expected result

- **Figure 14:** Use performance monitoring tool *perf* to measure system wide last level cache miss rate.

```
perf stat -e cycles,instruction,cache-misses,\
cache-references, bus-cycles -a sleep 10
```

### A.5 Experiment customization

- **Application level Timers:** We used the default timers of NPB and Nek5000 for each application.
- **Instruction level timers:** For Table 1 and Figure 5 in our papers, more accurate timers are needed to measure clflush performance. Modern processors makes it difficult to measure the elapsed time of individual instructions because of out-or-order execution of timer instructions. We use code in Fig 1 to achieve accurate measurement. Line 7 is the instructions to be measured.
- **Generate a larger eddy problem**: By default, the input problem eddy for Nek5000 is not big enough for multi-node execution. We generated a larger eddy problem using the Nek5000 tools, *genbox* and *genmap*.
  - Edit *eddy/eddy_uv.box* to increase problem size. (nelx=256,nely=256)

```
//New eddy_uv.box,base.rea and SIZE files are
    provided at the gitlab repo.

//Regenerate Nek5000 tools
cd Nek5000/tools
./maketools genmap && ./maketools genbox

// Generate new eddy_uv.rea with base.rea
//and eddy_uv.box provided
genbox
        eddy_uv.box
mv box.rea eddy_uv.rea
//generate new eddy_uv.map file
genmap
    eddy_uv
//Make executable for later experiments
makenek eddy_uv

```

**Figure 2.** Generating a larger eddy problem for Nek5000.

  - Edit *eddy/SIZE* to increase the preset limit of Nek program(e.g. max total number of elements(lelg), max number of mpi rank(lp) etc.).
  - Edit file *SIZE* in tools/genbox and tools/genmap to increase preset limit of Nek5000 tools.
  - To facilitate the user to execute the program, codes of new problem size are provided in Nek5000/run/eddy/ at the gitlab repo.
  - See Figure 2 for the workflow

### A.6 Experiment workflow

- Install and load the Quartz emulator and wbinvd kernel module; set desire emulated memory bandwdith.
- Choose target data objects and persistence establishment point for your application. For those applications with application-level checkpoint, the checkpointed data objects are the target data objects, and where the checkpoint happens is the persistence establishment point.
- Instrument the application with the LLVM-tracer and run the first iteration of the main computation loop in the application to generate a trace.
- Run our trace analysis tool over the trace to detect post-update version switch and nonuniform update. The tool outputs the statements where the first update and nonuniform updates happen.
- Run the code transformation tool using the trace analysis output and application source code as input.
- Insert flush_async() into the persistence establishment point within the application; insert flush_init() in front of the main computation loop of the application; insert flush_barrier() into the place where cache flush must finish within the application.
- Compile the application and link it with our runtime library for asynchronous and proactive cache flushing.
- Observe application output and measure performance.
